# Supplementary material for: Improving Label Error Detection and Elimination with Uncertainty Quantification
Source: arXiv:2405.09602 source file (2024-05-15)
Supplement: Supplementary file 1 [file 9_1_appendix_step_1.tex]

% =====================================================
\subsection{Step 1}
\label{apx:step1}
% =====================================================

% ================================
\paragraph*{\mnist Dataset}
% ================================

In \cref{tab:step1-mnist-performance-difference}, we report the difference in F1 score, precision, and recall of our algorithms compared to the baseline. 
The largest increase in average F1 score of 4.1\% is realized by the \clmcde algorithm. 
\begin{table}[h]
\centering
\labelerrorperformancedifferencetablecaption{2}{\mnist}{}
\label{tab:step1-mnist-performance-difference}
\setlength{\tabcolsep}{3pt}
\resizebox{\textwidth}{!}{%
\begin{tabular}{lcccccccccccc}
\hline
\multicolumn{1}{l|}{Measure}           & \multicolumn{4}{c|}{F1}                                                                                     & \multicolumn{4}{c|}{Precision}                                                                              & \multicolumn{4}{c}{Recall}                                                             \\
\multicolumn{1}{l|}{Noise Rate $\tau$} & 0.05           & 0.1            & \multicolumn{1}{c|}{0.2}            & \multicolumn{1}{c|}{$\Bar{X}$}      & 0.05           & 0.1            & \multicolumn{1}{c|}{0.2}            & \multicolumn{1}{c|}{$\Bar{X}$}      & 0.05           & 0.1            & \multicolumn{1}{c|}{0.2}            & $\Bar{X}$      \\ \hline
\multicolumn{1}{l|}{\clmcd}            & +1.6\%          & -0.3\%          & \multicolumn{1}{c|}{+1.6\%}          & \multicolumn{1}{c|}{+1.0\%}          & +3.8\%          & +2.0\%          & \multicolumn{1}{c|}{+1.5\%}          & \multicolumn{1}{c|}{+2.4\%}          & -0.4\%          & -2.3\%          & \multicolumn{1}{c|}{+1.8\%}          & -0.3\%          \\
\multicolumn{1}{l|}{\clmcde}           & \textbf{+3.7\%} & \textbf{+3.9\%} & \multicolumn{1}{c|}{\textbf{+4.8\%}} & \multicolumn{1}{c|}{\textbf{+4.1\%}} & +1.2\%          & +1.9\%          & \multicolumn{1}{c|}{\textbf{+6.3\%}} & \multicolumn{1}{c|}{+3.1\%}          & \textbf{+6.4\%} & \textbf{+5.8\%} & \multicolumn{1}{c|}{+3.7\%}          & \textbf{+5.3\%} \\
\multicolumn{1}{l|}{\clmcdme}          & +1.0\%          & -1.3\%          & \multicolumn{1}{c|}{-1.0\%}          & \multicolumn{1}{c|}{-0.4\%}          & +4.5\%          & \textbf{+3.2\%} & \multicolumn{1}{c|}{+3.2\%}          & \multicolumn{1}{c|}{+3.6\%}          & -2.2\%          & -5.3\%          & \multicolumn{1}{c|}{-4.6\%}          & -4.0\%          \\
\multicolumn{1}{l|}{\clmcdens}         & +3.4\%          & +2.0\%          & \multicolumn{1}{c|}{+2.9\%}          & \multicolumn{1}{c|}{+2.8\%}          & +3.7\%          & +2.0\%          & \multicolumn{1}{c|}{+2.2\%}          & \multicolumn{1}{c|}{+2.6\%}          & +3.1\%          & +2.0\%          & \multicolumn{1}{c|}{+3.7\%}          & +2.9\%          \\
\multicolumn{1}{l|}{\clalgens{2}}      & +2.6\%          & +2.5\%          & \multicolumn{1}{c|}{+3.1\%}          & \multicolumn{1}{c|}{+2.7\%}          & +3.1\%          & +2.3\%          & \multicolumn{1}{c|}{+1.7\%}          & \multicolumn{1}{c|}{+2.4\%}          & +2.2\%          & +2.5\%          & \multicolumn{1}{c|}{\textbf{+4.6\%}} & +3.1\%          \\
\multicolumn{1}{l|}{\clalgens{3}}      & +1.7\%          & +0.1\%          & \multicolumn{1}{c|}{+1.8\%}          & \multicolumn{1}{c|}{+1.2\%}          & \textbf{+4.6\%} & +3.1\%          & \multicolumn{1}{c|}{+4.9\%}          & \multicolumn{1}{c|}{\textbf{+4.2\%}} & -0.7\%          & -2.5\%          & \multicolumn{1}{c|}{-0.8\%}          & -1.3\%          \\ \hline
                                        & \multicolumn{3}{r}{Average:}                                           & +2.0\%                               & \multicolumn{3}{r}{Average:}                                           & +2.8\%                               & \multicolumn{3}{r}{Average:}                                           & +1.4\%         
\end{tabular}%
}
\end{table}

% ================================
\paragraph*{\cifarten Dataset}
% ================================
In \cref{tab:step1-cifar10-performance-difference}, we report the difference in F1 score, precision, and recall of our algorithms compared to the baseline. 
The better performance of our algorithms is mainly due to the substantial increase in precision at a similar or slightly reduced recall compared to the baseline.

\begin{table}[h]
\centering
\labelerrorperformancedifferencetablecaption{2}{\cifarten}{}
\label{tab:step1-cifar10-performance-difference}
\setlength{\tabcolsep}{3pt}
\resizebox{\textwidth}{!}{%
\begin{tabular}{lcccccccccccc}
\hline
\multicolumn{1}{l|}{Measure}           & \multicolumn{4}{c|}{F1}                                                                                     & \multicolumn{4}{c|}{Precision}                                                                                  & \multicolumn{4}{c}{Recall}                                                            \\
\multicolumn{1}{l|}{Noise Rate $\tau$} & 0.05           & 0.1            & \multicolumn{1}{c|}{0.2}            & \multicolumn{1}{c|}{$\Bar{X}$}      & 0.05            & 0.1             & \multicolumn{1}{c|}{0.2}             & \multicolumn{1}{c|}{$\Bar{X}$}       & 0.05           & 0.1           & \multicolumn{1}{c|}{0.2}            & $\Bar{X}$      \\ \hline
\multicolumn{1}{l|}{\clmcd}            & -0.7\%          & +0.4\%          & \multicolumn{1}{c|}{-0.2\%}          & \multicolumn{1}{c|}{-0.2\%}          & +0.3\%           & +0.8\%           & \multicolumn{1}{c|}{+0.1\%}           & \multicolumn{1}{c|}{+0.4\%}           & -2.5\%          & -0.3\%         & \multicolumn{1}{c|}{-0.5\%}          & -1.1\%          \\
\multicolumn{1}{l|}{\clmcde}           & \textbf{+8.7\%} & \textbf{+4.8\%} & \multicolumn{1}{c|}{\textbf{+4.0\%}} & \multicolumn{1}{c|}{\textbf{+5.8\%}} & \textbf{+18.6\%} & +11.4\%          & \multicolumn{1}{c|}{+9.3\%}           & \multicolumn{1}{c|}{+13.1\%}          & -3.8\%          & -2.7\%         & \multicolumn{1}{c|}{-1.5\%}          & -2.7\%          \\
\multicolumn{1}{l|}{\clmcdme}          & +5.6\%          & +1.4\%          & \multicolumn{1}{c|}{-8.8\%}          & \multicolumn{1}{c|}{-0.6\%}          & +14.9\%          & \textbf{+14.6\%} & \multicolumn{1}{c|}{\textbf{+10.2\%}} & \multicolumn{1}{c|}{\textbf{+13.2\%}} & -6.3\%          & -11.8\%        & \multicolumn{1}{c|}{-24.0\%}         & -14.0\%         \\
\multicolumn{1}{l|}{\clmcdens}         & -1.0\%          & 0.0\%           & \multicolumn{1}{c|}{-0.1\%}          & \multicolumn{1}{c|}{-0.4\%}          & 0.0\%            & +0.1\%           & \multicolumn{1}{c|}{+0.3\%}           & \multicolumn{1}{c|}{+0.1\%}           & -2.5\%          & \textbf{0.0\%} & \multicolumn{1}{c|}{-0.4\%}          & -1.0\%          \\
\multicolumn{1}{l|}{\clalgens{2}}      & -0.3\%          & +0.6\%          & \multicolumn{1}{c|}{+0.1\%}          & \multicolumn{1}{c|}{+0.1\%}          & +1.0\%           & +1.4\%           & \multicolumn{1}{c|}{+0.4\%}           & \multicolumn{1}{c|}{+0.9\%}           & \textbf{-2.2\%} & -0.3\%         & \multicolumn{1}{c|}{\textbf{-0.1\%}} & \textbf{-0.9\%} \\
\multicolumn{1}{l|}{\clalgens{3}}      & +5.9\%          & +4.6\%          & \multicolumn{1}{c|}{+3.4\%}          & \multicolumn{1}{c|}{+4.6\%}          & +12.3\%          & +11.3\%          & \multicolumn{1}{c|}{\textbf{+10.2\%}} & \multicolumn{1}{c|}{+11.3\%}          & -2.9\%          & -2.9\%         & \multicolumn{1}{c|}{-3.4\%}          & -3.1\%          \\ \hline
                                        & \multicolumn{3}{r}{Average:}                                           & +0.9\%                               & \multicolumn{3}{r}{Average:}                                              & +5.5\%                                & \multicolumn{3}{r}{Average:}                                          & -3.9\%         
\end{tabular}%
}
\end{table}

\FloatBarrier

% ================================
\paragraph*{\cifaronehundred Dataset}
% ================================
In \cref{tab:step1-cifar100-performance-difference}, we report the difference in F1 score, precision, and recall of our algorithms compared to the baseline. 
Contrary to all other algorithms, the performance of the \clmcdme declines with rising noise rates  due to a sharply declining recall which is up to 79.3\% lower than the baseline. 
Although it exhibits  the highest gains in precision among all algorithms of up to 127.9\%, the \clmcdme algorithm only achieves a better F1 score than the baseline at $\tau_1=0.05$. 

\begin{table}[h]
\centering
\labelerrorperformancedifferencetablecaption{2}{\cifaronehundred}{}
\label{tab:step1-cifar100-performance-difference}
\setlength{\tabcolsep}{3pt}
\resizebox{\textwidth}{!}{%
\begin{tabular}{lcccccccccccc}
\hline
\multicolumn{1}{l|}{Measure}           & \multicolumn{4}{c|}{F1}                                                                                        & \multicolumn{4}{c|}{Precision}                                                                                    & \multicolumn{4}{c}{Recall}                                                            \\
\multicolumn{1}{l|}{Noise Rate $\tau$} & 0.05            & 0.1             & \multicolumn{1}{c|}{0.2}            & \multicolumn{1}{c|}{$\Bar{X}$}       & 0.05             & 0.1              & \multicolumn{1}{c|}{0.2}             & \multicolumn{1}{c|}{$\Bar{X}$}       & 0.05           & 0.1            & \multicolumn{1}{c|}{0.2}           & $\Bar{X}$      \\ \hline
\multicolumn{1}{l|}{\clmcd}            & +3.9\%           & +2.3\%           & \multicolumn{1}{c|}{0.0\%}           & \multicolumn{1}{c|}{+2.1\%}           & +5.2\%            & +3.3\%            & \multicolumn{1}{c|}{+1.0\%}           & \multicolumn{1}{c|}{+3.2\%}           & 0.0\%           & -0.6\%          & \multicolumn{1}{c|}{-1.4\%}         & -0.7\%          \\
\multicolumn{1}{l|}{\clmcde}           & +12.8\%          & +8.6\%           & \multicolumn{1}{c|}{+3.2\%}          & \multicolumn{1}{c|}{+8.2\%}           & +20.3\%           & +16.9\%           & \multicolumn{1}{c|}{+11.4\%}          & \multicolumn{1}{c|}{+16.2\%}          & -11.2\%         & -9.3\%          & \multicolumn{1}{c|}{-8.1\%}         & -9.5\%          \\
\multicolumn{1}{l|}{\clmcdme}          & \textbf{+20.6\%} & -8.6\%           & \multicolumn{1}{c|}{-54.4\%}         & \multicolumn{1}{c|}{-14.1\%}          & \textbf{+127.9\%} & \textbf{+104.6\%} & \multicolumn{1}{c|}{\textbf{+52.8\%}} & \multicolumn{1}{c|}{\textbf{+95.1\%}} & -61.0\%         & -63.4\%         & \multicolumn{1}{c|}{-79.3\%}        & -67.9\%         \\
\multicolumn{1}{l|}{\clmcdens}         & +3.9\%           & +2.0\%           & \multicolumn{1}{c|}{-0.2\%}          & \multicolumn{1}{c|}{+1.9\%}           & +4.7\%            & +2.3\%            & \multicolumn{1}{c|}{-0.2\%}           & \multicolumn{1}{c|}{+2.3\%}           & \textbf{+2.1\%} & \textbf{+1.2\%} & \multicolumn{1}{c|}{\textbf{0.0\%}} & \textbf{+1.1\%} \\
\multicolumn{1}{l|}{\clalgens{2}}      & +3.9\%           & +2.3\%           & \multicolumn{1}{c|}{+0.8\%}          & \multicolumn{1}{c|}{+2.3\%}           & +5.8\%            & +3.6\%            & \multicolumn{1}{c|}{+1.8\%}           & \multicolumn{1}{c|}{+3.7\%}           & -2.1\%          & -1.7\%          & \multicolumn{1}{c|}{-1.0\%}         & -1.6\%          \\
\multicolumn{1}{l|}{\clalgens{3}}      & +19.1\%          & \textbf{+10.7\%} & \multicolumn{1}{c|}{\textbf{+3.7\%}} & \multicolumn{1}{c|}{\textbf{+11.2\%}} & +31.4\%           & +24.2\%           & \multicolumn{1}{c|}{+17.3\%}          & \multicolumn{1}{c|}{+24.3\%}          & -15.3\%         & -14.8\%         & \multicolumn{1}{c|}{-13.5\%}        & -14.5\%         \\ \hline
                                        & \multicolumn{3}{r}{Average:}                                             & +0.1\%                                & \multicolumn{3}{r|}{Average:}                                               & +24.1\%                               & \multicolumn{3}{r}{Average:}                                          & -15.7\%        
\end{tabular}%
}
\end{table}

% ================================
\paragraph*{\tinyimagenet Dataset}
% ================================
In \cref{tab:step1-tiny-imagenet-performance-difference}, we report the difference in F1 score, precision, and recall of our algorithms compared to the baseline. 
We generally observe that the F1 score of all algorithms increases with higher noise rates, except for the \clmcdme algorithm.
Although the precision of the \clmcdme algorithm is the highest among all algorithms, its overall label error detection performance on the \tinyimagenet is worse than that of the baseline. 
The reason for the weak performance of the \clmcdme algorithm is again its poor recall, which is up to 81.0\% lower than the baseline.

\begin{table}[h]
\centering
\labelerrorperformancedifferencetablecaption{2}{\tinyimagenet}{}
\label{tab:step1-tiny-imagenet-performance-difference}
\setlength{\tabcolsep}{3pt}
\resizebox{\textwidth}{!}{%
\begin{tabular}{lcccccccccccc}
\hline
\multicolumn{1}{l|}{Measure}           & \multicolumn{4}{c|}{F1}                                                                                        & \multicolumn{4}{c|}{Precision}                                                                                     & \multicolumn{4}{c}{Recall}                                                             \\
\multicolumn{1}{l|}{Noise Rate $\tau$} & 0.05            & 0.1             & \multicolumn{1}{c|}{0.2}            & \multicolumn{1}{c|}{$\Bar{X}$}       & 0.05             & 0.1              & \multicolumn{1}{c|}{0.2}             & \multicolumn{1}{c|}{$\Bar{X}$}        & 0.05           & 0.1            & \multicolumn{1}{c|}{0.2}            & $\Bar{X}$      \\ \hline
\multicolumn{1}{l|}{\clmcd}            & +7.0\%           & +3.7\%           & \multicolumn{1}{c|}{+0.7\%}          & \multicolumn{1}{c|}{+3.8\%}           & +8.1\%            & +5.3\%            & \multicolumn{1}{c|}{+1.9\%}           & \multicolumn{1}{c|}{+5.1\%}            & -0.5\%          & -0.1\%          & \multicolumn{1}{c|}{-2.1\%}          & -0.9\%          \\
\multicolumn{1}{l|}{\clmcde}           & +17.4\%          & +10.1\%          & \multicolumn{1}{c|}{+3.1\%}          & \multicolumn{1}{c|}{+10.2\%}          & +23.0\%           & +17.5\%           & \multicolumn{1}{c|}{+12.6\%}          & \multicolumn{1}{c|}{+17.7\%}           & -8.6\%          & -8.9\%          & \multicolumn{1}{c|}{-12.0\%}         & -9.8\%          \\
\multicolumn{1}{l|}{\clmcdme}          & -7.8\%           & -17.7\%          & \multicolumn{1}{c|}{-42.5\%}         & \multicolumn{1}{c|}{-22.7\%}          & \textbf{+167.4\%} & \textbf{+140.2\%} & \multicolumn{1}{c|}{\textbf{+79.6\%}} & \multicolumn{1}{c|}{\textbf{+129.1\%}} & -81.0\%         & -74.0\%         & \multicolumn{1}{c|}{-75.7\%}         & -76.9\%         \\
\multicolumn{1}{l|}{\clmcdens}         & +7.8\%           & +3.4\%           & \multicolumn{1}{c|}{+0.9\%}          & \multicolumn{1}{c|}{+4.0\%}           & +8.1\%            & +3.7\%            & \multicolumn{1}{c|}{+0.7\%}           & \multicolumn{1}{c|}{+4.2\%}            & \textbf{+5.8\%} & \textbf{+3.2\%} & \multicolumn{1}{c|}{\textbf{+1.1\%}} & \textbf{+3.4\%} \\
\multicolumn{1}{l|}{\clalgens{2}}      & +9.6\%           & +5.3\%           & \multicolumn{1}{c|}{+1.5\%}          & \multicolumn{1}{c|}{+5.5\%}           & +11.1\%           & +6.9\%            & \multicolumn{1}{c|}{+3.4\%}           & \multicolumn{1}{c|}{+7.1\%}            & +0.5\%          & +0.4\%          & \multicolumn{1}{c|}{-1.8\%}          & -0.3\%          \\
\multicolumn{1}{l|}{\clalgens{3}}      & \textbf{+21.7\%} & \textbf{+13.0\%} & \multicolumn{1}{c|}{\textbf{+3.6\%}} & \multicolumn{1}{c|}{\textbf{+12.8\%}} & +33.3\%           & +28.9\%           & \multicolumn{1}{c|}{+21.8\%}          & \multicolumn{1}{c|}{+28.0\%}           & -20.6\%         & -19.5\%         & \multicolumn{1}{c|}{-20.2\%}         & -20.1\%         \\ \hline
                                        & \multicolumn{3}{r}{Average:}                                             & +0.2\%                                & \multicolumn{3}{r}{Average:}                                                & +32.6\%                                & \multicolumn{3}{r}{Average:}                                           & -16.9\%        
\end{tabular}%
}
\end{table}
