# Supplementary material for: Improving Label Error Detection and Elimination with Uncertainty Quantification
Source: arXiv:2405.09602 source file (2024-05-15)
Supplement: Supplementary file 2 [file 9_2_appendix_step_2.tex]

% =====================================================
\subsection{Step 2}
\label{apx:step2}
% =====================================================

% ================================
\paragraph*{\mnist Dataset}
% ================================
In \cref{tab:mnist-performance-difference}, we report the percentage difference in F1 score, precision, and recall between our algorithms and the baseline.
All our proposed uncertainty-based algorithms achieve a better F1 score across all noise rates than the baseline, except for the \clmcde and \clalgens{3} at $\tau_3=0.2$. 
Across all noise rates, the application of our algorithms leads to an increase in precision of 3.2\% on average, while the recall is reduced by  1.1\% on average. 

\begin{table}[h]
\centering
\labelerrorperformancedifferencetablecaption{2}{\mnist}{}
\label{tab:mnist-performance-difference}
\resizebox{\textwidth}{!}{%
\begin{tabular}{lcccccccccccc}
\hline
\multicolumn{1}{l|}{Measure}                     & \multicolumn{4}{c|}{F1}                                                                                         & \multicolumn{4}{c|}{Precision}                                                                                  & \multicolumn{4}{c}{Recall}                                                                 \\
\multicolumn{1}{l|}{Noise Rate $\tau$}           & 0.05            & 0.1             & \multicolumn{1}{c|}{0.2}             & \multicolumn{1}{c|}{$\Bar{X}$}       & 0.05            & 0.1             & \multicolumn{1}{c|}{0.2}             & \multicolumn{1}{c|}{$\Bar{X}$}       & 0.05            & 0.1             & \multicolumn{1}{c|}{0.2}             & $\Bar{X}$       \\ \hline
\multicolumn{1}{l|}{\clmcd}                      & +1.6\%          & +1.1\%          & \multicolumn{1}{c|}{+0.6\%}          & \multicolumn{1}{c|}{+1.1\%}          & +3.9\%          & +3.2\%          & \multicolumn{1}{c|}{+2.7\%}          & \multicolumn{1}{c|}{+3.3\%}          & -0.6\%          & -0.7\%          & \multicolumn{1}{c|}{-1.3\%}          & -0.9\%          \\
\multicolumn{1}{l|}{\clmcde}                  & +1.4\%          & +0.4\%          & \multicolumn{1}{c|}{-2.2\%}          & \multicolumn{1}{c|}{-0.1\%}          & +2.5\%          & +2.9\%          & \multicolumn{1}{c|}{+2.6\%}          & \multicolumn{1}{c|}{+2.7\%}          & +0.2\%          & -1.8\%          & \multicolumn{1}{c|}{-6.6\%}          & -2.7\%          \\
\multicolumn{1}{l|}{\clmcdens}             & +1.6\%          & +1.4\%          & \multicolumn{1}{c|}{+0.6\%}          & \multicolumn{1}{c|}{+1.2\%}          & +2.9\%          & +2.4\%          & \multicolumn{1}{c|}{+2.4\%}          & \multicolumn{1}{c|}{+2.6\%}          & +0.2\%          & +0.3\%          & \multicolumn{1}{c|}{-1.0\%}          & -0.2\%          \\
\multicolumn{1}{l|}{\clalgens{2}} & \textbf{+2.3\%} & \textbf{+2.1\%} & \multicolumn{1}{c|}{\textbf{+1.6\%}} & \multicolumn{1}{c|}{\textbf{+2.0\%}} & +3.5\%          & +3.2\%          & \multicolumn{1}{c|}{+2.3\%}          & \multicolumn{1}{c|}{+3.0\%}          & \textbf{+1.2\%} & \textbf{+1.2\%} & \multicolumn{1}{c|}{\textbf{+1.0\%}} & \textbf{+1.1\%} \\
\multicolumn{1}{l|}{\clalgens{3}} & +2.0\%          & +0.7\%          & \multicolumn{1}{c|}{-1.1\%}          & \multicolumn{1}{c|}{+0.5\%}          & \textbf{+5.0\%} & \textbf{+4.2\%} & \multicolumn{1}{c|}{\textbf{+4.0\%}} & \multicolumn{1}{c|}{\textbf{+4.4\%}} & -0.9\%          & -2.3\%          & \multicolumn{1}{c|}{-5.5\%}          & -2.9\%          \\ \hline
                                                 & \multicolumn{3}{r}{Average:}                                             & +0.9\%                               & \multicolumn{3}{r}{Average:}                                             & +3.2\%                               & \multicolumn{3}{r}{Average:}                                             & -1.1\%         
\end{tabular}%
}
\end{table}

In \cref{fig:mnist-accuracy-comparison-noisy}, we depict the differences in accuracy before and after cleaning the \mnist training set with the different algorithms.
We observe no notable differences between the noisy accuracy and the clean accuracies achieved by the different algorithms. 
The largest increase in accuracy of 0.5\% is achieved by the \clmcde algorithm at $\tau_3=0.5$.

\begin{figure}[h]%
\centering
\includegraphics[width=0.9\textwidth]{1_Figures/step2_results/mnist/perc_accuracy_noisy.jpg}
\accuracydifferencesnoisycaption{2}{\mnist}{}%Read: At noise rate $\tau_1=0.05$ cleaning with the \clmcde algorithm increases the test set accuracy by 0.2\%.
\label{fig:mnist-accuracy-comparison-noisy}
\end{figure}

\clearpage

In \cref{fig:mnist-number-label-errors-comparison}, we report the percentage difference between the number of potential label errors found and removed by the baseline and our algorithms.
We observe that the large majority of our algorithms achieve slightly better accuracies compared to the baseline (see \cref{fig:mnist-accuracy-comparison-noisy}) while removing fewer potential label errors.

\begin{figure}[h]%
\centering
\includegraphics[width=0.9\textwidth]{1_Figures/step2_results/mnist/perc_number_of_label_errors.jpg}
\labelerrorremoveddifferencescaption{2}{\mnist}{}
\label{fig:mnist-number-label-errors-comparison}
\end{figure}

\FloatBarrier

% ================================
\paragraph*{\cifarten Dataset}
% ================================
In \cref{tab:cifar-10-performance-difference}, we report the percentage difference in F1 score, precision, and recall between our algorithms and the baseline.
The results show that our proposed uncertainty-based methods perform notably better than the baseline \clpbnr method. 
The better label error detection performance of our algorithms is due to the greatly increased precision. 
On average, we observe an increase in precision of 28.2\% across all noise rates and algorithms, while the recall only marginally deteriorates by 2.8\% on average across all noise rates.

\begin{table}[h]
\centering
\labelerrorperformancedifferencetablecaption{2}{\cifarten}{}
\label{tab:cifar-10-performance-difference}
\setlength{\tabcolsep}{3pt}
\resizebox{\textwidth}{!}{%
\begin{tabular}{lcccccccccccc}
\hline
\multicolumn{1}{l|}{Measure}                     & \multicolumn{4}{c|}{F1}                                                                                             & \multicolumn{4}{c|}{Precision}                                                                                      & \multicolumn{4}{c|}{Recall}                                                                                     \\
\multicolumn{1}{l|}{Noise Rate $\tau$}           & 0.05             & 0.1              & \multicolumn{1}{c|}{0.2}              & \multicolumn{1}{c|}{$\Bar{X}$}        & 0.05             & 0.1              & \multicolumn{1}{c|}{0.2}              & \multicolumn{1}{c|}{$\Bar{X}$}        & 0.05            & 0.1             & \multicolumn{1}{c|}{0.2}             & \multicolumn{1}{c|}{$\Bar{X}$}       \\ \hline
\multicolumn{1}{l|}{\clmcd}                      & +24.1\%          & +13.9\%          & \multicolumn{1}{c|}{+5.1\%}           & \multicolumn{1}{c|}{+14.4\%}          & +38.6\%          & +24.1\%          & \multicolumn{1}{c|}{+10.3\%}          & \multicolumn{1}{c|}{+24.3\%}          & -3.5\%          & -3.1\%          & \multicolumn{1}{c|}{-2.4\%}          & \multicolumn{1}{c|}{-3.0\%}          \\
\multicolumn{1}{l|}{\clmcde}                  & \textbf{+37.1\%} & \textbf{+27.5\%} & \multicolumn{1}{c|}{\textbf{+15.1\%}} & \multicolumn{1}{c|}{\textbf{+26.6\%}} & \textbf{+65.3\%} & \textbf{+52.1\%} & \multicolumn{1}{c|}{\textbf{+30.0\%}} & \multicolumn{1}{c|}{\textbf{+49.1\%}} & -6.5\%          & -5.5\%          & \multicolumn{1}{c|}{-4.0\%}          & \multicolumn{1}{c|}{-5.3\%}          \\
\multicolumn{1}{l|}{\clmcdens}             & +7.5\%           & +5.5\%           & \multicolumn{1}{c|}{+3.3\%}           & \multicolumn{1}{c|}{+5.4\%}           & +10.1\%          & +7.3\%           & \multicolumn{1}{c|}{+4.2\%}           & \multicolumn{1}{c|}{+7.2\%}           & \textbf{+0.9\%} & \textbf{+1.5\%} & \multicolumn{1}{c|}{\textbf{+1.6\%}} & \multicolumn{1}{c|}{\textbf{+1.3\%}} \\
\multicolumn{1}{l|}{\clalgens{2}} & +24.1\%          & +14.8\%          & \multicolumn{1}{c|}{+6.8\%}           & \multicolumn{1}{c|}{+15.2\%}          & +38.0\%          & +24.8\%          & \multicolumn{1}{c|}{+11.3\%}          & \multicolumn{1}{c|}{+24.7\%}          & -2.7\%          & -1.9\%          & \multicolumn{1}{c|}{-0.2\%}          & \multicolumn{1}{c|}{-1.6\%}          \\
\multicolumn{1}{l|}{\clalgens{3}} & +29.8\%          & +19.6\%          & \multicolumn{1}{c|}{+9.6\%}           & \multicolumn{1}{c|}{+19.7\%}          & +50.7\%          & +36.7\%          & \multicolumn{1}{c|}{+20.3\%}          & \multicolumn{1}{c|}{+35.9\%}          & -6.0\%          & -5.7\%          & \multicolumn{1}{c|}{-5.0\%}          & \multicolumn{1}{c|}{-5.6\%}          \\ \hline
                                                 & \multicolumn{3}{r}{Average:}                                                & +16.3\%                               & \multicolumn{3}{r}{Average:}                                                & +28.2\%                               & \multicolumn{3}{r}{Average:}                                             & -2.8\%                              
\end{tabular}%
}
\end{table}

\clearpage

In \cref{fig:cifar10-accuracy-comparison-noisy}, we depict the differences in accuracy before and after cleaning the \cifarten training set with the different algorithms.
All algorithms achieve substantial accuracy gains at all noise rates compared to the noisy dataset. 
The achieved accuracy gains of the algorithms increase with higher noise rates. 

\begin{figure}[h!]%
\centering
\includegraphics[width=0.9\textwidth]{1_Figures/step2_results/cifar10/perc_accuracy_noisy.jpg}
\accuracydifferencesnoisycaption{2}{\cifarten}{} % Read: At noise rate $\tau_1=0.05$, cleaning with the \clmcde algorithm increases the test set accuracy by 3.8\%.
\label{fig:cifar10-accuracy-comparison-noisy}
\end{figure}

\FloatBarrier

% ================================
\paragraph*{\cifaronehundred Dataset}
% ================================

In \cref{tab:cifar-100-performance-difference}, we report the percentage difference in F1 score, precision, and recall between our algorithms and the baseline.
We observe that all our uncertainty-based algorithms perform better in terms of F1 score than the baseline.
The higher performance of our algorithms can be attributed to an increase in precision of up to 55.3\% for the \clalgens{3}, at $\tau_1=0.05$. 
On average, the precision increases by 22.5\% while the recall decreases by 6.7\% across all noise rates and algorithms. 

\begin{table}[h]
\centering
\labelerrorperformancedifferencetablecaption{2}{\cifaronehundred}{}
\label{tab:cifar-100-performance-difference}
\setlength{\tabcolsep}{3pt}
\resizebox{\textwidth}{!}{%
\begin{tabular}{lcccccccccccc}
\hline
\multicolumn{1}{l|}{Measure}                     & \multicolumn{4}{c|}{F1}                                                                                             & \multicolumn{4}{c|}{Precision}                                                                                      & \multicolumn{4}{c}{Recall}                                                                 \\
\multicolumn{1}{l|}{Noise Rate $\tau$}           & 0.05             & 0.1              & \multicolumn{1}{c|}{0.2}              & \multicolumn{1}{c|}{$\Bar{X}$}        & 0.05             & 0.1              & \multicolumn{1}{c|}{0.2}              & \multicolumn{1}{c|}{$\Bar{X}$}        & 0.05            & 0.1             & \multicolumn{1}{c|}{0.2}             & $\Bar{X}$       \\ \hline
\multicolumn{1}{l|}{\clmcd}                      & +16.8\%          & +10.6\%          & \multicolumn{1}{c|}{+6.2\%}           & \multicolumn{1}{c|}{+11.2\%}          & +21.3\%          & +15.5\%          & \multicolumn{1}{c|}{+10.6\%}          & \multicolumn{1}{c|}{+15.8\%}          & -4.2\%          & -4.1\%          & \multicolumn{1}{c|}{-3.6\%}          & -4.0\%          \\
\multicolumn{1}{l|}{\clmcde}                  & +33.2\%          & +20.2\%          & \multicolumn{1}{c|}{+10.5\%}          & \multicolumn{1}{c|}{+21.3\%}          & +45.4\%          & +33.5\%          & \multicolumn{1}{c|}{+23.2\%}          & \multicolumn{1}{c|}{+34.0\%}          & -13.6\%         & -12.0\%         & \multicolumn{1}{c|}{-11.4\%}         & -12.3\%         \\
\multicolumn{1}{l|}{\clmcdens}             & +2.9\%           & +2.1\%           & \multicolumn{1}{c|}{+1.5\%}           & \multicolumn{1}{c|}{+2.2\%}           & +3.5\%           & +2.0\%           & \multicolumn{1}{c|}{+0.8\%}           & \multicolumn{1}{c|}{+2.1\%}           & \textbf{+2.9\%} & \textbf{+3.1\%} & \multicolumn{1}{c|}{\textbf{+3.4\%}} & \textbf{+3.1\%} \\
\multicolumn{1}{l|}{\clalgens{2}} & +20.1\%          & +12.7\%          & \multicolumn{1}{c|}{+7.5\%}           & \multicolumn{1}{c|}{+13.4\%}          & +24.8\%          & +18.4\%          & \multicolumn{1}{c|}{+12.1\%}          & \multicolumn{1}{c|}{+18.4\%}          & -4.4\%          & -4.0\%          & \multicolumn{1}{c|}{-2.6\%}          & -3.7\%          \\
\multicolumn{1}{l|}{\clalgens{3}} & \textbf{+38.1\%} & \textbf{+23.8\%} & \multicolumn{1}{c|}{\textbf{+11.6\%}} & \multicolumn{1}{c|}{\textbf{+24.5\%}} & \textbf{+55.3\%} & \textbf{+42.0\%} & \multicolumn{1}{c|}{\textbf{+29.0\%}} & \multicolumn{1}{c|}{\textbf{+42.1\%}} & -18.1\%         & -16.1\%         & \multicolumn{1}{c|}{-15.9\%}         & -16.7\%         \\ \hline
                                                 & \multicolumn{3}{r}{Average:}                                                & +14.5\%                               & \multicolumn{3}{r}{Average:}                                                & +22.5\%                               & \multicolumn{3}{r}{Average:}                                             & -6.7\%         
\end{tabular}%
}
\end{table}

\FloatBarrier

% ================================
\paragraph*{\tinyimagenet Dataset}
% ================================

In \cref{tab:tiny-imagenet-performance-difference}, we report the percentage difference in F1 score, precision, and recall between our algorithms and the baseline.
All our uncertainty-based algorithms perform better in terms of F1 score than the baseline (see \cref{fig:tiny-imagenet-f1-comparison}).
On average, the improvement in F1 score across all noise rates is at least 4.4\% and at most 19.6\% compared to the baseline.
The higher performance of our algorithms can be attributed to an overall increase in precision of up to 41.5\% for the \clalgens{3} at $\tau_1=0.05$. 
On average, the precision of our algorithms is 17.4\% higher than the baseline, while the recall is 4.5\% lower. 

\begin{table}[h]
\centering
\labelerrorperformancedifferencetablecaption{2}{\tinyimagenet}{}
\label{tab:tiny-imagenet-performance-difference}
\setlength{\tabcolsep}{3pt}
\resizebox{\textwidth}{!}{%
\begin{tabular}{lcccccccccccc}
\hline
\multicolumn{1}{l|}{Measure}                     & \multicolumn{4}{c|}{F1}                                                                                             & \multicolumn{4}{c|}{Precision}                                                                                      & \multicolumn{4}{c|}{Recall}                                                                                     \\
\multicolumn{1}{l|}{Noise Rate $\tau$}           & 0.05             & 0.1              & \multicolumn{1}{c|}{0.2}              & \multicolumn{1}{c|}{$\Bar{X}$}        & 0.05             & 0.1              & \multicolumn{1}{c|}{0.2}              & \multicolumn{1}{c|}{$\Bar{X}$}        & 0.05            & 0.1             & \multicolumn{1}{c|}{0.2}             & \multicolumn{1}{c|}{$\Bar{X}$}       \\ \hline
\multicolumn{1}{l|}{\clmcd}                      & +9.3\%           & +5.6\%           & \multicolumn{1}{c|}{+4.4\%}           & \multicolumn{1}{c|}{+6.4\%}           & +11.5\%          & +8.3\%           & \multicolumn{1}{c|}{+7.4\%}           & \multicolumn{1}{c|}{+9.1\%}           & -1.6\%          & -2.7\%          & \multicolumn{1}{c|}{-1.2\%}          & \multicolumn{1}{c|}{-1.8\%}          \\
\multicolumn{1}{l|}{\clmcde}                  & +20.9\%          & +15.0\%          & \multicolumn{1}{c|}{\textbf{+11.3\%}} & \multicolumn{1}{c|}{+15.7\%}          & +26.9\%          & +23.3\%          & \multicolumn{1}{c|}{+20.6\%}          & \multicolumn{1}{c|}{+23.6\%}          & -7.2\%          & -6.5\%          & \multicolumn{1}{c|}{-4.1\%}          & \multicolumn{1}{c|}{-5.9\%}          \\
\multicolumn{1}{l|}{\clmcdens}             & +5.8\%           & +3.7\%           & \multicolumn{1}{c|}{+3.6\%}           & \multicolumn{1}{c|}{+4.4\%}           & +6.2\%           & +4.6\%           & \multicolumn{1}{c|}{+3.9\%}           & \multicolumn{1}{c|}{+4.9\%}           & \textbf{+3.4\%} & \textbf{+1.9\%} & \multicolumn{1}{c|}{\textbf{+3.1\%}} & \multicolumn{1}{c|}{\textbf{+2.8\%}} \\
\multicolumn{1}{l|}{\clalgens{2}} & +13.8\%          & +9.4\%           & \multicolumn{1}{c|}{+7.1\%}           & \multicolumn{1}{c|}{+10.1\%}          & +16.9\%          & +13.3\%          & \multicolumn{1}{c|}{+11.1\%}          & \multicolumn{1}{c|}{+13.8\%}          & -1.7\%          & -2.0\%          & \multicolumn{1}{c|}{-0.2\%}          & \multicolumn{1}{c|}{-1.3\%}          \\
\multicolumn{1}{l|}{\clalgens{3}} & \textbf{+28.9\%} & \textbf{+19.0\%} & \multicolumn{1}{c|}{+10.9\%}          & \multicolumn{1}{c|}{\textbf{+19.6\%}} & \textbf{+41.5\%} & \textbf{+35.4\%} & \multicolumn{1}{c|}{\textbf{+29.2\%}} & \multicolumn{1}{c|}{\textbf{+35.4\%}} & -17.7\%         & -16.4\%         & \multicolumn{1}{c|}{-14.4\%}         & \multicolumn{1}{c|}{-16.2\%}         \\ \hline
                                                 & \multicolumn{3}{r}{Average:}                                                & +11.2\%                               & \multicolumn{3}{r}{Average:}                                                & +17.4\%                               & \multicolumn{3}{r}{Average:}                                             & -4.5\%                              
\end{tabular}%
}
\end{table}
\FloatBarrier

% ================================
\paragraph*{Average Label Error Detection Performance of All Algorithms}
% ================================

In \cref{tab:average-score-algorithms}, we report the average performance of all algorithms across the different datasets and noise rates. 
The percentage differences to the baseline can be found in \cref{tab:average-difference-score-algorithms}. 
Overall, all of our algorithms perform better than the baseline (\clpbnr) on average. 
As already noted in the results sections of the respective datasets, the reason for the higher label error detection performance (F1 score) of our algorithms is the higher precision at a slightly reduced recall. 

In general, the \clmcde algorithm and the \clalgens{3} achieve the highest label error detection performance, or F1 score, across all datasets (except the \mnist dataset) and noise rates. 
Both algorithms have the highest average precision of 55.4\% and 55.7\%, respectively. 
However, with 83.2\% and 80.0\%, their average recall is the lowest compared to all other algorithms. 
The highest average recall is achieved by the \clmcd ensemble with 90.6\% followed by the baseline (\clpbnr) with 89.1\%, the \clalgens{2} with 87.8\%, and the \clmcd algorithm with 86.9\%. 

\begin{sidewaystable}
\setlength{\tabcolsep}{3pt}
\caption[\protect\stepprefix{2}: Average label error detection performance of all algorithms per dataset]{Average label error detection performance of all algorithms per dataset.}
\label{tab:average-score-algorithms}
\resizebox{\textheight}{!}{%
\begin{tabular}{lccccccccccccccc}
\hline
\multicolumn{1}{l|}{Measure}      & \multicolumn{5}{c|}{Average F1 Score}                                                                                        & \multicolumn{5}{c|}{Average Precision Score}                                                                                 & \multicolumn{5}{c}{Average Recall Score}                                                                \\
\multicolumn{1}{l|}{Dataset}      & MNIST          & CIFAR-10       & CIFAR-100      & \multicolumn{1}{c|}{Tiny ImageNet}  & \multicolumn{1}{c|}{$\Bar{X}$}      & MNIST          & CIFAR-10       & CIFAR-100      & \multicolumn{1}{c|}{Tiny ImageNet}  & \multicolumn{1}{c|}{$\Bar{X}$}      & MNIST          & CIFAR-10       & CIFAR-100      & \multicolumn{1}{c|}{Tiny ImageNet}  & $\Bar{X}$      \\ \hline
\multicolumn{1}{l|}{\clpbnr}      & 94.2\%          & 55.2\%          & 38.8\%          & \multicolumn{1}{c|}{38.3\%}          & \multicolumn{1}{c|}{56.6\%}          & 94.0\%          & 40.8\%          & 25.5\%          & \multicolumn{1}{c|}{25.9\%}          & \multicolumn{1}{c|}{46.6\%}          & 94.4\%          & 87.5\%          & 90.3\%          & \multicolumn{1}{c|}{84.0\%}          & 89.1\%          \\
\multicolumn{1}{l|}{\clmcd}       & 95.2\%          & 62.8\%          & 42.6\%          & \multicolumn{1}{c|}{40.5\%}          & \multicolumn{1}{c|}{60.3\%}          & 97.0\%          & 50.1\%          & 29.1\%          & \multicolumn{1}{c|}{28.1\%}          & \multicolumn{1}{c|}{51.1\%}          & 93.5\%          & 84.8\%          & 86.7\%          & \multicolumn{1}{c|}{82.4\%}          & 86.9\%          \\
\multicolumn{1}{l|}{\clmcde}      & 94.0\%          & \textbf{69.5\%} & 46.0\%          & \multicolumn{1}{c|}{43.8\%}          & \multicolumn{1}{c|}{\textbf{63.3\%}} & 96.5\%          & \textbf{60.1\%} & 33.3\%          & \multicolumn{1}{c|}{31.7\%}          & \multicolumn{1}{c|}{55.4\%}          & 91.8\%          & 82.7\%          & 79.2\%          & \multicolumn{1}{c|}{79.0\%}          & 83.2\%          \\
\multicolumn{1}{l|}{\clmcdens}    & 95.3\%          & 58.2\%          & 39.6\%          & \multicolumn{1}{c|}{39.9\%}          & \multicolumn{1}{c|}{58.3\%}          & 96.4\%          & 43.6\%          & 25.9\%          & \multicolumn{1}{c|}{27.1\%}          & \multicolumn{1}{c|}{48.3\%}          & 94.2\%          & \textbf{88.6\%} & \textbf{93.2\%} & \multicolumn{1}{c|}{\textbf{86.3\%}} & \textbf{90.6\%} \\
\multicolumn{1}{l|}{\clalgens{2}} & \textbf{96.1\%} & 63.3\%          & 43.4\%          & \multicolumn{1}{c|}{41.8\%}          & \multicolumn{1}{c|}{61.2\%}          & 96.8\%          & 50.3\%          & 29.7\%          & \multicolumn{1}{c|}{29.2\%}          & \multicolumn{1}{c|}{51.5\%}          & \textbf{95.4\%} & 86.0\%          & 87.0\%          & \multicolumn{1}{c|}{82.9\%}          & 87.8\%          \\
\multicolumn{1}{l|}{\clalgens{3}} & 94.7\%          & 65.7\%          & \textbf{47.0\%} & \multicolumn{1}{c|}{\textbf{44.9\%}} & \multicolumn{1}{c|}{63.1\%}          & \textbf{98.1\%} & 54.8\%          & \textbf{35.2\%} & \multicolumn{1}{c|}{\textbf{34.5\%}} & \multicolumn{1}{c|}{\textbf{55.7\%}} & 91.6\%          & 82.6\%          & 75.3\%          & \multicolumn{1}{c|}{70.4\%}          & 80.0\%          \\ \hline
                                    & \multicolumn{4}{r}{Average:}                                                           & 60.5\%                               & \multicolumn{4}{r}{Average:}                                                           & 51.4\%                               & \multicolumn{4}{r}{Average:}                                                           & 86.3\%         
\end{tabular}%
}

\bigskip\bigskip\bigskip\bigskip\bigskip

\caption[\protect\stepprefix{2}: Difference in average label error detection performance per dataset between our algorithms and the baseline (\clpbnr)]{Difference in average label error detection performance per dataset between our algorithms and the baseline (\clpbnr).}
\label{tab:average-difference-score-algorithms}
\resizebox{\textwidth}{!}{%
\begin{tabular}{lccccccccccccccc}
\hline
\multicolumn{1}{l|}{Measure}                     & \multicolumn{5}{c|}{Difference in Average F1 Score}                                                                                                & \multicolumn{5}{c|}{Difference in Average Precision}                                                                                               & \multicolumn{5}{c}{Difference in Average Recall}                                                                            \\
\multicolumn{1}{l|}{Dataset}                     & \mnist                & \cifarten             & \cifaronehundred            & \multicolumn{1}{c|}{\tinyimagenet}    & \multicolumn{1}{c|}{$\Bar{X}$}        & \mnist                & \cifarten             & \cifaronehundred            & \multicolumn{1}{c|}{\tinyimagenet}    & \multicolumn{1}{c|}{$\Bar{X}$}        & \mnist                & \cifarten             & \cifaronehundred            & \multicolumn{1}{c|}{\tinyimagenet}   & $\Bar{X}$       \\ \hline
\multicolumn{1}{l|}{\clmcd}                      & +1.1\%               & +13.8\%              & +9.9\%               & \multicolumn{1}{c|}{+5.9\%}           & \multicolumn{1}{c|}{+7.7\%}           & +3.3\%               & +22.7\%              & +14.1\%              & \multicolumn{1}{c|}{+8.4\%}           & \multicolumn{1}{c|}{+12.1\%}          & -0.9\%               & -3.0\%               & -4.0\%               & \multicolumn{1}{c|}{-1.8\%}          & -2.4\%          \\
\multicolumn{1}{l|}{\clmcde}                  & -0.1\%               & \textbf{+25.8\%}     & +18.5\%              & \multicolumn{1}{c|}{+14.4\%}          & \multicolumn{1}{c|}{\textbf{+14.7\%}} & +2.7\%               & \textbf{+47.1\%}     & +30.6\%              & \multicolumn{1}{c|}{+22.5\%}          & \multicolumn{1}{c|}{+25.7\%}          & -2.7\%               & -5.4\%               & -12.4\%              & \multicolumn{1}{c|}{-5.9\%}          & -6.6\%          \\
\multicolumn{1}{l|}{\clmcdens}             & +1.2\%               & +5.3\%               & +2.0\%               & \multicolumn{1}{c|}{+4.1\%}           & \multicolumn{1}{c|}{+3.2\%}           & +2.6\%               & +6.9\%               & +1.7\%               & \multicolumn{1}{c|}{+4.5\%}           & \multicolumn{1}{c|}{+3.9\%}           & -0.1\%               & \textbf{+1.3\%}      & \textbf{+3.1\%}      & \multicolumn{1}{c|}{\textbf{+2.8\%}} & \textbf{+1.8\%} \\
\multicolumn{1}{l|}{\clalgens{2}} & \textbf{+2.0\%}      & +14.7\%              & +11.9\%              & \multicolumn{1}{c|}{+9.2\%}           & \multicolumn{1}{c|}{+9.5\%}           & +3.0\%               & +23.2\%              & +16.5\%              & \multicolumn{1}{c|}{+12.7\%}          & \multicolumn{1}{c|}{+13.9\%}          & \textbf{+1.1\%}      & -1.7\%               & -3.7\%               & \multicolumn{1}{c|}{-1.3\%}          & -1.4\%          \\
\multicolumn{1}{l|}{\clalgens{3}} & +0.6\%               & +19.0\%              & \textbf{+21.2\%}     & \multicolumn{1}{c|}{\textbf{+17.1\%}} & \multicolumn{1}{c|}{+14.5\%}          & \textbf{+4.4\%}      & +34.2\%              & \textbf{+38.0\%}     & \multicolumn{1}{c|}{\textbf{+33.3\%}} & \multicolumn{1}{c|}{\textbf{+27.5\%}} & -2.9\%               & -5.6\%               & -16.7\%              & \multicolumn{1}{c|}{-16.1\%}         & -10.3\%         \\ \hline
                                                 & \multicolumn{1}{l}{} & \multicolumn{1}{l}{} & \multicolumn{1}{l}{} & \multicolumn{1}{r}{Average:}          & +9.9\%                                & \multicolumn{1}{l}{} & \multicolumn{1}{l}{} & \multicolumn{1}{l}{} & \multicolumn{1}{r}{Average:}          & +16.6\%                               & \multicolumn{1}{l}{} & \multicolumn{1}{l}{} & \multicolumn{1}{l}{} & \multicolumn{1}{r}{Average:}         & -3.8\%         
\end{tabular}%
}
\end{sidewaystable}

\FloatBarrier

\paragraph*{Comparison of Results Between Step 1 and Step 2}
In \cref{tab:correlation-step-1-2-t-values}, we report the $t$-values of our test for the significance of the correlations between the F1 scores from \step{1} and \step{2} at a significance level of $\alpha=0.05$. 
The sample size $n$ corresponds to the number of different noise rates, i.e., $n=3$, and the degrees of freedom equals $df=n-2=1$. 
The $t$-values are calculated using the test statistic defined in \cref{subsec:comparison-step1-2},  \cref{test-statistic}. 
The corresponding $p$-values are presented in the main body of this work in \cref{tab:correlation-step-1-2}.

\begin{table}[h]
\centering
\caption[\protect\stepprefix{2}: Correlations between Step 1 and Step 2 ($t$-values)]{Correlations between the F1 Scores from \step{1} and \step{2} of our evaluation procedure of all algorithms across all noise rates together with the corresponding $t$-value.}
\label{tab:correlation-step-1-2-t-values}
\setlength{\tabcolsep}{3pt}
\resizebox{\textwidth}{!}{%
\begin{tabular}{l|cccc|cccc}
\hline
Measure      & \multicolumn{4}{c|}{Correlation Coefficient   $r$} & \multicolumn{4}{c}{$t$-value}                        \\
Dataset      & \mnist   & \cifarten   & \cifaronehundred   & \tinyimagenet   & \mnist & \cifarten & \cifaronehundred & \tinyimagenet \\ \hline
\clpbnr      & -0.75    & 1.00        & 1.00               & 1.00            & 1.13   & 10.11     & 36.75            & 159.40        \\
\clmcd       & 0.97     & 0.91        & 1.00               & 1.00            & 3.78   & 2.22      & 34.79            & 41.04         \\
\clmcde      & 0.94     & 0.63        & 1.00               & 1.00            & 2.84   & 0.82      & 29.68            & 30.68         \\
\clmcdme     & -        & -           & -                  & -               & -      & -         & -                & -             \\
\clmcdens    & 0.95     & 1.00        & 1.00               & 1.00            & 3.10   & 15.76     & 60.39            & 56.55         \\
\clalgens{2} & 0.97     & 0.97        & 1.00               & 1.00            & 3.78   & 3.84      & 25.57            & 45.54         \\
\clalgens{3} & 0.98     & 0.84        & 1.00               & 1.00            & 5.59   & 1.54      & 15.99            & 36.03         \\ \hline
\end{tabular}%
}
\end{table}

\FloatBarrier
% ================================
\paragraph*{Effects of Replacing Softmax with Monte-Carlo Dropout Probabilities - An Example}
\label{subsec:precision-example}
% ================================

In the discussion chapter, we argued that replacing softmax probabilities with \ac{MCD} probabilities leads to better precision of our label error detection algorithms compared to the baseline.
To better understand this, we will explain the effects of using \ac{MCD} predictions instead of softmax predictions with an example. 
Given a dataset $\pmb{X}$ with four classes, so $\mathcal{K} :=\{ \text{\enquote{SUV}},  \text{\enquote{Pickup}}, \text{\enquote{Truck}}, \text{\enquote{Motorcycle}}\}$, a model $\pmb{\theta}$ predicts the softmax and \ac{MCD} probabilities defined in \cref{example-predictions} for a sample $\pmb{x} \in \pmb{X}$.

\begin{table}[h]
\begin{center}
\caption[Example: Softmax and \ac{MCD} probabilities]{Softmax and \ac{MCD} probabilities for sample $x$.}
\label{example-predictions}
\setlength{\tabcolsep}{15pt}

\begin{tabular}{|c|c|c|c|c|}
\hline
$\bm{j}$                          & \textbf{SUV} & \textbf{Pickup} & \textbf{Truck} & \textbf{Motorcycle} \\ \hline
$\hat{p}_{\pmb{x},\Tilde{y}=j}$              & 80\%         & 15\%            & 4\%            & 1\%                 \\ \hline
$\hat{p}^{\text{MCD}}_{\pmb{x},\Tilde{y}=j}$ & 50\%         & 48\%            & 1\%            & 1\%                 \\ \hline
\end{tabular}%
\end{center}
\end{table}

The given label of $\pmb{x}$ is $\Tilde{y}=\text{\enquote{Pickup}}$. 
We assume that this label is correct, i.e., $\Tilde{y}=y^{*}=\text{\enquote{Pickup}}$. 
The threshold $t_j$, i.e., average predicted probability of all samples belonging to class $j \in \mathcal{K}$, (see \cref{subsec:confident_learning}, \cref{eq:cl-threshold}) is reported in \cref{example-threshold}. 

\begin{table}[h]
\begin{center}
\caption[Example: Threshold $t_j$]{Thresholds $t_j$ of our exemplary dataset $\pmb{X}$.}
\label{example-threshold}
\setlength{\tabcolsep}{15pt}

\begin{tabular}{|c|c|c|c|c|}
\hline
$\bm{j}$  & \textbf{SUV} & \textbf{Pickup} & \textbf{Truck} & \textbf{Motorcycle} \\ \hline
$t_j$                & 75\%         & 82\%            & 90\%            & 80\%                 \\ \hline
\end{tabular}%
\end{center}
\end{table}

Considering only the softmax predictions, we conclude that the model is very \enquote{certain} that the given label $\Tilde{y}=\text{\enquote{Pickup}}$ is wrong and that the actual label should be in fact $y^{*}=\text{\enquote{SUV}}$. 
Regarding the threshold in the first \ac{CL} step (\enquote{Count}), $t_\text{SUV}=75\% < \hat{p}_{\pmb{x},\Tilde{y}=\text{SUV}}=80\%$ holds, and consequently, the sample is falsely counted as a label error in the confident joint. 
The precision of the label error detection algorithm reduces.
If we look at the \ac{MCD} probabilities instead, it becomes clear that the model is uncertain whether the sample belongs to class $j=\text{\enquote{SUV}}$ or $j=\text{\enquote{Pickup}}$.  
The model's prediction is still $\hat{y}=\text{\enquote{SUV}}$, but only with a probability of $\hat{p}^{\text{MCD}}_{\pmb{x},\Tilde{y}=\text{SUV}}=50\%$. 
This probability is below the threshold $t_\text{SUV}=75\%$, and consequently, the sample is not counted as a label error in the confident joint. 
The precision of the label error detection algorithm does not decline.
Consequently, using \ac{MCD} instead of softmax probabilities results in a better precision of our label error detection algorithms compared to the baseline.

\FloatBarrier
