# Supplementary material for: Improving Label Error Detection and Elimination with Uncertainty Quantification
Source: arXiv:2405.09602 source file (2024-05-15)
Supplement: Supplementary file 3 [file 9_3_appendix_low_noise.tex]

% =====================================================
\subsection{Low Noise Study}
\label{apx:low-noise-study}
% =====================================================

% ================================
\paragraph*{\cifarten Dataset}
% ================================
In \cref{tab:cifar10-performance-difference-low-noise}, we report the percentage difference in F1 score, precision, and recall between our algorithms and the baseline.
We can observe that our algorithms perform substantially better than the baseline \clpbnr algorithm. 
The average improvement in performance across all noise rates is at least 9.3\% and at most 51.8\% compared to the baseline.

\begin{table}[h]
\centering
\labelerrorperformancedifferencetablecaption{3}{\cifarten}{}
\label{tab:cifar10-performance-difference-low-noise}
\setlength{\tabcolsep}{3pt}
\resizebox{\textwidth}{!}{%
\begin{tabular}{lcccccccccccc}
\hline
\multicolumn{1}{l|}{Measure}                       & \multicolumn{4}{c|}{F1}                                                                                             & \multicolumn{4}{c|}{Precision}                                                                                      & \multicolumn{4}{c}{Recall}                                                   \\
\multicolumn{1}{l|}{Noise Rate $\tau$}             & 0.02             & 0.03             & \multicolumn{1}{c|}{0.04}             & \multicolumn{1}{c|}{$\Bar{X}$}        & 0.02             & 0.03             & \multicolumn{1}{c|}{0.04}             & \multicolumn{1}{c|}{$\Bar{X}$}        & 0.02            & 0.03            & \multicolumn{1}{c|}{0.04}            & $\Bar{X}$       \\ \hline
\multicolumn{1}{l|}{\clmcd}                        & +41.7\%          & +31.0\%          & \multicolumn{1}{c|}{+29.0\%}          & \multicolumn{1}{c|}{+33.9\%}          & +58.8\%          & +46.9\%          & \multicolumn{1}{c|}{+44.9\%}          & \multicolumn{1}{c|}{+50.2\%}          & -3.9\%          & -4.6\%          & \multicolumn{1}{c|}{-3.2\%}          & -3.9\%          \\
\multicolumn{1}{l|}{\clmcde}                    & \textbf{+62.1\%} & \textbf{+48.8\%} & \multicolumn{1}{c|}{\textbf{+44.6\%}} & \multicolumn{1}{c|}{\textbf{+51.8\%}} & \textbf{+94.8\%} & \textbf{+78.8\%} & \multicolumn{1}{c|}{\textbf{+75.4\%}} & \multicolumn{1}{c|}{\textbf{+83.0\%}} & -6.5\%          & -6.7\%          & \multicolumn{1}{c|}{-5.6\%}          & -6.3\%          \\
\multicolumn{1}{l|}{\clmcdme}                   & +42.9\%          & +32.8\%          & \multicolumn{1}{c|}{+29.9\%}          & \multicolumn{1}{c|}{+35.2\%}          & +61.1\%          & +50.4\%          & \multicolumn{1}{c|}{+48.2\%}          & \multicolumn{1}{c|}{+53.2\%}          & -4.7\%          & -5.6\%          & \multicolumn{1}{c|}{-5.2\%}          & -5.2\%          \\
\multicolumn{1}{l|}{\clmcdens}             & +12.0\%          & +8.1\%           & \multicolumn{1}{c|}{+7.7\%}           & \multicolumn{1}{c|}{+9.3\%}           & +14.2\%          & +10.8\%          & \multicolumn{1}{c|}{+10.3\%}          & \multicolumn{1}{c|}{+11.8\%}          & \textbf{+1.7\%} & \textbf{+0.2\%} & \multicolumn{1}{c|}{\textbf{+1.0\%}} & \textbf{+1.0\%} \\
\multicolumn{1}{l|}{\clalgens{2}} & +40.2\%          & +30.8\%          & \multicolumn{1}{c|}{+28.8\%}          & \multicolumn{1}{c|}{+33.3\%}          & +56.4\%          & +45.8\%          & \multicolumn{1}{c|}{+44.5\%}          & \multicolumn{1}{c|}{+48.9\%}          & -3.3\%          & -3.9\%          & \multicolumn{1}{c|}{-2.7\%}          & -3.3\%          \\
\multicolumn{1}{l|}{\clalgens{3}} & +50.4\%          & +39.2\%          & \multicolumn{1}{c|}{+36.7\%}          & \multicolumn{1}{c|}{+42.1\%}          & +73.5\%          & +61.2\%          & \multicolumn{1}{c|}{+59.5\%}          & \multicolumn{1}{c|}{+64.7\%}          & -5.2\%          & -5.6\%          & \multicolumn{1}{c|}{-4.5\%}          & -5.1\%          \\ \hline
                                                   & \multicolumn{3}{r}{Average:}                                                & +34.3\%                                & \multicolumn{3}{r}{Average:}                                                & +52.0\%                                & \multicolumn{3}{r}{Average:}                                             & -3.8\%         
\end{tabular}%
}
\end{table}

\FloatBarrier

% ================================
\paragraph*{\cifaronehundred Dataset}
% ================================

In \cref{tab:cifar100-performance-difference-low-noise}, we report the percentage difference in F1 score, precision, and recall between our algorithms and the baseline.
All our algorithms perform considerably better in terms of F1 score than the baseline. 
In this setting, it is the first time that neither the \clmcde algorithm nor the \clalgens{3} achieve the best label error detection performance across all noise rates but the \clmcdme algorithm. 
It achieves an average boost in F1 score of 66.8\% compared to the baseline. 

\begin{table}[h]
\centering
\labelerrorperformancedifferencetablecaption{3}{\cifaronehundred}{}
\label{tab:cifar100-performance-difference-low-noise}
\setlength{\tabcolsep}{3pt}
\resizebox{\textwidth}{!}{%
\begin{tabular}{lcccccccccccc}
\hline
\multicolumn{1}{l|}{Measure}                       & \multicolumn{4}{c|}{F1}                                                                                             & \multicolumn{4}{c|}{Precision}                                                                                         & \multicolumn{4}{c}{Recall}                                                                 \\
\multicolumn{1}{l|}{Noise Rate $\tau$}             & 0.02             & 0.03             & \multicolumn{1}{c|}{0.04}             & \multicolumn{1}{c|}{$\Bar{X}$}        & 0.02              & 0.03              & \multicolumn{1}{c|}{0.04}             & \multicolumn{1}{c|}{$\Bar{X}$}         & 0.02            & 0.03            & \multicolumn{1}{c|}{0.04}            & $\Bar{X}$       \\ \hline
\multicolumn{1}{l|}{\clmcd}                        & +20.0\%          & +19.6\%          & \multicolumn{1}{c|}{+18.9\%}          & \multicolumn{1}{c|}{+19.5\%}          & +23.9\%           & +22.6\%           & \multicolumn{1}{c|}{+23.3\%}          & \multicolumn{1}{c|}{+23.3\%}           & -7.4\%          & -4.7\%          & \multicolumn{1}{c|}{-4.6\%}          & -5.6\%          \\
\multicolumn{1}{l|}{\clmcde}                    & +43.2\%          & +42.3\%          & \multicolumn{1}{c|}{+35.8\%}          & \multicolumn{1}{c|}{+40.4\%}          & +52.2\%           & +52.7\%           & \multicolumn{1}{c|}{+48.3\%}          & \multicolumn{1}{c|}{+51.1\%}           & -17.3\%         & -13.3\%         & \multicolumn{1}{c|}{-15.2\%}         & -15.3\%         \\
\multicolumn{1}{l|}{\clmcdme}                   & \textbf{+72.0\%} & \textbf{+72.6\%} & \multicolumn{1}{c|}{\textbf{+55.7\%}} & \multicolumn{1}{c|}{\textbf{+66.8\%}} & \textbf{+100.0\%} & \textbf{+109.7\%} & \multicolumn{1}{c|}{\textbf{+97.5\%}} & \multicolumn{1}{c|}{\textbf{+102.4\%}} & -39.2\%         & -35.9\%         & \multicolumn{1}{c|}{-39.1\%}         & -38.1\%         \\
\multicolumn{1}{l|}{\clmcdens}             & +3.2\%           & +3.6\%           & \multicolumn{1}{c|}{+3.8\%}           & \multicolumn{1}{c|}{+3.5\%}           & +3.0\%            & +3.2\%            & \multicolumn{1}{c|}{+4.2\%}           & \multicolumn{1}{c|}{+3.5\%}            & \textbf{+2.6\%} & \textbf{+4.5\%} & \multicolumn{1}{c|}{\textbf{+4.4\%}} & \textbf{+3.8\%} \\
\multicolumn{1}{l|}{\clalgens{2}} & +25.6\%          & +25.0\%          & \multicolumn{1}{c|}{+21.7\%}          & \multicolumn{1}{c|}{+24.1\%}          & +29.9\%           & +29.0\%           & \multicolumn{1}{c|}{+26.7\%}          & \multicolumn{1}{c|}{+28.5\%}           & -7.4\%          & -4.3\%          & \multicolumn{1}{c|}{-5.3\%}          & -5.7\%          \\
\multicolumn{1}{l|}{\clalgens{3}} & +52.0\%          & +49.4\%          & \multicolumn{1}{c|}{+42.5\%}          & \multicolumn{1}{c|}{+48.0\%}          & +64.2\%           & +62.4\%           & \multicolumn{1}{c|}{+58.3\%}          & \multicolumn{1}{c|}{+61.6\%}           & -20.8\%         & -17.4\%         & \multicolumn{1}{c|}{-18.7\%}         & -19.0\%         \\ \hline
                                                    & \multicolumn{3}{r}{Average:}                                                & +33.7\%                                & \multicolumn{3}{r}{Average:}                                                  & +45.1\%                                 & \multicolumn{3}{r}{Average:}                                             & -13.3\%        
\end{tabular}%
}
\end{table}
\FloatBarrier
